# Supplementary material for: Understanding Reader Takeaways in Thematic Maps Under Varying Text, Detail, and Spatial Autocorrelation
Source: arXiv:2403.08260 source file (2024-03-13)
Supplement: Supplementary file 1 [file 9_supplemental.tex]

\section*{Supplemental Materials}
\label{sec:supplemental_materials}

All supplemental materials are available on OSF at \url{https://osf.io/3pzvj/?view_only=86167a2f0ba041899f6edee0c73c6f68}, released under a xxxxxxxxxxxx license.
In particular, they include (1) source code of the study, (2) original stimuli images and (3) analyses scripts. This is a anonymous, read-only link for the purposes of review only.
